# Supplementary material for: UniMPA: A Unified Memory-Prediction-Action Model via Action-Grounded Transition Modeling
Source: arXiv:2609.11875 source file (2026-09-10)
Supplement: Supplementary file 1 [file supp-robotwin.tex]

\begin{table*}[htbp]
\centering
\caption{
Per-task success rates on the 50 RoboTwin 2.0 tasks under
the Randomized setting.
}
\label{tab:robotwin_random_50results}
\setlength{\tabcolsep}{2.6pt}
\renewcommand{\arraystretch}{1.08}
\resizebox{\textwidth}{!}{%
\begin{tabular}{l|cccccccccccc}
\toprule
\multirow{2}{*}{\textit{Task}}
& ACT~\cite{zhao2023act}
& DP~\cite{diff}
& DP3~\cite{ze20243d}
& RDT~\cite{liu2024rdt}
& $\pi_0$~\cite{pi0}
& UP-VLA~\cite{zhang2025up}
& ADV~\cite{zhao2026action}
& TwinVLA~\cite{im2025twinvla}
& BagelVLA~\cite{hu2026bagelvla}
& HALO~\cite{shou2026halo}
& $\pi_{0.5}$~\cite{pi05}
& \multirow{2}{*}{\textbf{UniMPA}} \\

& \textit{[RSS'23]}
& \textit{[RSS'23]}
& \textit{[RSS'24]}
& \textit{[ICLR'25]}
& \textit{[RSS'25]}
& \textit{[ICML'25]}
& \textit{[arXiv'26]}
& \textit{[ICLR'26]}
& \textit{[RSS'26]}
& \textit{[ICML'26]}
& \textit{[arXiv'25]}
& \\
\midrule

\textit{Adjust Bottle}
& 23\% & 0\% & 3\% & 75\% & 56\% & 17\% & 26\%
& 35\% & 14\% & 9\% & 54\% & \textbf{80\%} \\

\textit{Beat Block Hammer}
& 3\% & 0\% & 8\% & \textbf{37\%} & 21\% & 16\% & 0\%
& 10\% & 16\% & 11\% & 0\% & 24\% \\

\textit{Blocks Ranking RGB}
& 0\% & 0\% & 0\% & 0\% & 5\% & 0\% & \textbf{24\%}
& 0\% & 4\% & 7\% & 8\% & 8\% \\

\textit{Blocks Ranking Size}
& 0\% & 0\% & 0\% & 0\% & 1\% & 0\% & 0\%
& 0\% & 2\% & 2\% & \textbf{11\%} & 4\% \\

\textit{Click Alarmclock}
& 4\% & 5\% & 14\% & 12\% & 11\% & 41\% & 22\%
& 1\% & 20\% & 14\% & \textbf{62\%} & 28\% \\

\textit{Click Bell}
& 3\% & 0\% & 0\% & 9\% & 3\% & 72\% & 13\%
& 13\% & 35\% & 10\% & \textbf{85\%} & 24\% \\

\textit{Dump Bin Bigbin}
& 1\% & 0\% & 53\% & 32\% & 24\% & 35\% & 15\%
& 34\% & 51\% & 28\% & 30\% & \textbf{62\%} \\

\textit{Grab Roller}
& 25\% & 0\% & 2\% & 43\% & 80\% & 28\% & 46\%
& 22\% & 41\% & 57\% & 63\% & \textbf{84\%} \\

\textit{Handover Block}
& 0\% & 0\% & 0\% & 14\% & 8\% & 0\% & 6\%
& 0\% & 0\% & \textbf{36\%} & 0\% & 12\% \\

\textit{Handover Mic}
& 0\% & 0\% & 3\% & 31\% & 13\% & 0\% & 2\%
& 2\% & 8\% & \textbf{61\%} & 2\% & 34\% \\

\textit{Hanging Mug}
& 0\% & 0\% & 1\% & \textbf{16\%} & 3\% & 0\% & 0\%
& 5\% & 1\% & 5\% & 1\% & 3\% \\

\textit{Lift Pot}
& 0\% & 0\% & 0\% & 9\% & \textbf{36\%} & 0\% & 9\%
& 7\% & 32\% & 34\% & 0\% & 8\% \\

\textit{Move Can Pot}
& 4\% & 0\% & 6\% & 12\% & \textbf{21\%} & 0\% & 11\%
& 5\% & 0\% & 15\% & 0\% & 13\% \\

\textit{Move Pillbottle Pad}
& 0\% & 0\% & 0\% & 0\% & 1\% & 7\% & 1\%
& 2\% & 1\% & \textbf{26\%} & 20\% & 15\% \\

\textit{Move Playingcard Away}
& 0\% & 0\% & 3\% & 11\% & 22\% & 13\% & 17\%
& 35\% & 30\% & \textbf{53\%} & 14\% & 46\% \\

\textit{Move Stapler Pad}
& 0\% & 0\% & 0\% & 0\% & 2\% & 0\% & 0\%
& 0\% & 0\% & \textbf{19\%} & 4\% & 8\% \\

\textit{Open Laptop}
& 0\% & 0\% & 7\% & 32\% & 46\% & 21\% & 27\%
& 17\% & 37\% & 37\% & 3\% & \textbf{67\%} \\

\textit{Open Microwave}
& 0\% & 0\% & 22\% & 20\% & \textbf{50\%} & 7\% & 39\%
& 1\% & 0\% & 24\% & 14\% & 24\% \\

\textit{Pick Diverse Bottles}
& 0\% & 0\% & 1\% & 0\% & 6\% & 18\% & 2\%
& 8\% & \textbf{34\%} & 17\% & 14\% & 18\% \\

\textit{Pick Dual Bottles}
& 0\% & 0\% & 1\% & 13\% & 12\% & 31\% & 9\%
& 12\% & \textbf{56\%} & 30\% & 20\% & 25\% \\

\textit{Place A2B Left}
& 0\% & 0\% & 2\% & 1\% & 1\% & 4\% & 0\%
& 5\% & 12\% & 8\% & 12\% & \textbf{20\%} \\

\textit{Place A2B Right}
& 0\% & 0\% & 0\% & 1\% & 6\% & 1\% & 0\%
& 1\% & 11\% & 9\% & 6\% & \textbf{14\%} \\

\textit{Place Bread Basket}
& 0\% & 0\% & 1\% & 2\% & 4\% & 20\% & 2\%
& 3\% & 29\% & 26\% & \textbf{38\%} & 31\% \\

\textit{Place Bread Skillet}
& 0\% & 0\% & 0\% & 1\% & 1\% & 16\% & 1\%
& 1\% & \textbf{26\%} & 23\% & 19\% & 16\% \\

\textit{Place Burger Fries}
& 0\% & 0\% & 18\% & 27\% & 4\% & 26\% & 11\%
& 13\% & 11\% & 37\% & \textbf{45\%} & 40\% \\

\textit{Place Can Basket}
& 0\% & 0\% & 2\% & 6\% & 5\% & 0\% & 2\%
& 0\% & 0\% & \textbf{34\%} & 7\% & 17\% \\

\textit{Place Cans Plasticbox}
& 0\% & 0\% & 3\% & 5\% & 2\% & 24\% & 0\%
& 8\% & 5\% & \textbf{47\%} & 27\% & 18\% \\

\textit{Place Container Plate}
& 1\% & 0\% & 1\% & 17\% & 45\% & 48\% & 11\%
& 4\% & 58\% & 22\% & 58\% & \textbf{75\%} \\

\textit{Place Dual Shoes}
& 0\% & 0\% & 0\% & 4\% & 0\% & 0\% & 0\%
& 3\% & 0\% & 3\% & 3\% & \textbf{7\%} \\

\textit{Place Empty Cup}
& 0\% & 0\% & 1\% & 7\% & 11\% & 27\% & 3\%
& 1\% & 34\% & 28\% & 53\% & \textbf{57\%} \\

\textit{Place Fan}
& 0\% & 0\% & 1\% & 2\% & 10\% & 1\% & 1\%
& 0\% & 5\% & 9\% & 8\% & \textbf{19\%} \\

\textit{Place Mouse Pad}
& 0\% & 0\% & 1\% & 0\% & 1\% & 0\% & 0\%
& 0\% & \textbf{14\%} & 12\% & 11\% & 6\% \\

\textit{Place Object Basket}
& 0\% & 0\% & 0\% & 17\% & 2\% & 1\% & 4\%
& 3\% & 3\% & \textbf{25\%} & \textbf{25\%} & 16\% \\

\textit{Place Object Scale}
& 0\% & 0\% & 0\% & 0\% & 0\% & 4\% & 0\%
& 0\% & 0\% & 5\% & 20\% & \textbf{38\%} \\

\textit{Place Object Stand}
& 0\% & 0\% & 0\% & 5\% & 11\% & 24\% & 0\%
& 2\% & 21\% & 33\% & 45\% & \textbf{59\%} \\

\textit{Place Phone Stand}
& 0\% & 0\% & 2\% & 6\% & 7\% & 0\% & 6\%
& 2\% & 2\% & 10\% & 7\% & \textbf{37\%} \\

\textit{Place Shoe}
& 0\% & 0\% & 2\% & 7\% & 6\% & 12\% & 2\%
& 4\% & 29\% & 18\% & 41\% & \textbf{49\%} \\

\textit{Press Stapler}
& 6\% & 0\% & 3\% & 24\% & 29\% & 56\% & 15\%
& 26\% & 58\% & 64\% & \textbf{72\%} & 67\% \\

\textit{Put Bottles Dustbin}
& 1\% & 0\% & \textbf{21\%} & 4\% & 13\% & 0\% & 9\%
& 4\% & 10\% & 13\% & 10\% & 18\% \\

\textit{Put Object Cabinet}
& 0\% & 0\% & 1\% & \textbf{18\%} & \textbf{18\%} & 0\% & 0\%
& 16\% & 0\% & 8\% & 7\% & 15\% \\

\textit{Rotate QRCode}
& 0\% & 0\% & 1\% & 5\% & 15\% & 2\% & 9\%
& 3\% & 21\% & 11\% & 10\% & \textbf{22\%} \\

\textit{Scan Object}
& 0\% & 0\% & 1\% & 1\% & 1\% & 23\% & 0\%
& 4\% & \textbf{32\%} & 24\% & 7\% & 20\% \\

\textit{Shake Bottle Horizontally}
& 4\% & 18\% & 25\% & 51\% & 51\% & 68\% & 42\%
& 55\% & 73\% & 66\% & 94\% & \textbf{95\%} \\

\textit{Shake Bottle}
& 10\% & 8\% & 19\% & 45\% & 60\% & 54\% & 37\%
& 58\% & 74\% & 73\% & \textbf{96\%} & 94\% \\

\textit{Stack Blocks Three}
& 0\% & 0\% & 0\% & 0\% & 0\% & 0\% & 0\%
& 0\% & 5\% & \textbf{37\%} & 14\% & 1\% \\

\textit{Stack Blocks Two}
& 0\% & 0\% & 0\% & 2\% & 1\% & 0\% & 2\%
& 0\% & 6\% & \textbf{60\%} & 33\% & 6\% \\

\textit{Stack Bowls Three}
& 0\% & 0\% & 5\% & 17\% & 24\% & 1\% & 26\%
& 15\% & 13\% & 25\% & 24\% & \textbf{38\%} \\

\textit{Stack Bowls Two}
& 0\% & 0\% & 6\% & 30\% & 41\% & 12\% & 48\%
& 11\% & 52\% & 49\% & 52\% & \textbf{69\%} \\

\textit{Stamp Seal}
& 0\% & 0\% & 0\% & 0\% & 4\% & 2\% & 0\%
& 1\% & 8\% & 21\% & 15\% & \textbf{24\%} \\

\textit{Turn Switch}
& 2\% & 1\% & 8\% & 15\% & 23\% & 26\% & 9\%
& 15\% & 30\% & 27\% & 20\% & \textbf{34\%} \\

\midrule
\textbf{\textit{Average}}
& 1.74\% & 0.64\% & 4.96\% & 13.72\% & 16.34\%
& 15.16\% & 10.20\% & 9.34\% & 20.48\%
& 26.44\% & 25.68\% & \textbf{32.18\%} \\
\bottomrule
\end{tabular}
}
\end{table*}
